# Supplementary material for: Towards Knowledge-Based Recommender Dialog System
Source: arXiv:1908.05391 source file (2019-09-03)
Supplement: Supplementary file 1 [file appendix.tex]

\section{Supplemental Material}
